# Supplementary material for: Top-k Query Processing on Encrypted Databases with Strong Security Guarantees
Source: arXiv:1510.05175 source file (2018-01-18)
Supplement: Supplementary file 1 [file appendix.tex]

\begin{appendices}
\section{Security between $S_1$ and $S_2$}\label{app:servers-security}

Informally, our privacy definitions capture the following: 
$S_1$ learns the number of documents and the halting depth, as well as the query pattern and access pattern of client queries since he observes the ``encrypted'' queries of the client. 
However, $S_1$ learns nothing about the objects and scores as they are all protected by the semantic encryption scheme. 
$S_2$, on the other hand, only learns the equality pattern at each depth when executing the protocol $\SecQuery$ with $S_1$. 
In other words, the cryptography cloud $S_2$ learns some pattern from the encrypted data when the client is querying the system. 
However, $S_2$ learns nothing about the access and query patterns, and hence does not know anything about how does $S_1$ access the encrypted relation, nor the content of the queries. 
We note that $S_1$'s capabilities are similar to those of the server in the original searchable encryption and structured encryption definition~\cite{CGKO06, CK10} while $S_2$ learns much less. 

We formalize the privacy between the semi-honest adversaries $S_1$ and $S_2$ as follows: 
Let $\Pi_f$ be a two-party protocol that supports the functionality $f$
during the query processing. 
Let $\view_{S_i}^{\Pi_f}(I)$ be all the transcripts that $S_i$ receives 
while running the protocol on input $I$, 
and let $\SIM_{s_i}$ be the simulator who tries to simulate the views for $S_i$. 
While executing the protocol, let $\SIM_{s_i}(\L_{s_i}(\cdot))$ denote the simulated 
transcript by $\SIM_{s_i}$ on the input $\L_{s_i}(\cdot)$, 
where $\L_{s_i}(\cdot)$ is a stateful function that $\SIM_{s_i}$ learns during 
the execution of the protocol.
At the beginning, $S_1$ has the encrypted database $\ER$ and the 
public key $\pk$, while $S_2$ holds the public/secret key $\pk$ and $\sk$. 

\begin{definition}\label{def:sec-servers}
Let $\Pi_f$ be a two party protocol for computing a function $f$. 
$S_1$ takes the input $(\pk_\p, x)$ and $S_2$ takes the input $(\pk_\p, \sk_\p, y)$.
When $\Pi_f$ terminates $S_1$ receives $f(x, y)$. 
Let $\view^{\Pi_f}_{S_i}(\pk_\p, \sk_\p, x, y)$ be all the message that $S_i$
receives while running the protocol on input $(\pk_\p, \sk_\p, x, y)$ and 
$\oput^{f}$ be the output of the protocol received by $S_1$.
We say that the protocol $\Pi_f$ between $S_1$ and $S_2$  privately realizes 
the functionality $f$ if there exists a pair of probabilistic polynomial time (PPT) 
simulators $\SIM_{s_1}$ and $\SIM_{s_2}$ such that: 
\begin{align*}
(1). \Big(\SIM_{s_2}\big(\pk_\p, \L_{s_2}\big), \Pi_f(\pk_\p, \sk_\p, x, y) \Big) & \approxeq \Big(\view^{\Pi_f}_{S_1}(\pk_\p, \sk_\p, x, y),  \oput^{f}(\pk_\p, \sk_\p , x, y)\Big)\\
(2).  \Big(\SIM_{s_1}\big(\pk_\p, \sk_\p, \L_{s_1}\big) & \approxeq \view_{S_2}^{\Pi_f}(\pk_\p, \sk_\p, x, y)\Big)
\end{align*} 
\end{definition}

%Here we formally define the leakage during the query execution.
%For any query $q$, suppose there are $m$ number of objects at each depth, then
%\begin{itemize}
%\item \emph{Equality pattern $\EP^d(\ER, q)$:}
%         On input of $\ER$ and a query $q$, at depth $d$ of $\ER$, $\EP^d(\ER, q)$ outputs a symmetric binary $m\times m$ matrix $M^d$, where $M^d[i, j] = 0$ if there exist objects $o_{\pi(i')} = o_{\pi(j')}$ for some random permutation $\pi$ such that $\pi(i')=i$ and $\pi(j')=j$. Otherwise, $M^d[i, j] = 0$.
%\end{itemize}
%Note that $\EP^d(\ER, q)$ does not leak the equality relations between objects at any depth in the original database, 
%i.e. the server never knows which objects are same since the server does not know the permutation.
The two sub-routines $\EncSort$ and $\EncCompare$ have been proved to be secure 
in~\cite{fc15/FO, DBLP:conf/ndss/BostPTG15} 
and we refer the proofs from there. 
Below we show that $\SecWorst$ we describe in the section~\ref{subsec:secworst} is secure based on the security definition~\ref{def:sec-servers}. In addition, the security of $\SecBest$, $\SecDedup$, $\SecUpdate$ are very similar to the proof of $\SecWorst$.

\begin{lemma}\label{lemma:secworst}
Let $\SecWorst$ be the protocol between $S_1$ and $S_2$ described in Algorithm~\ref{alg:sec-worst} that privately computes the $\SecWorst$ functionality at depth $d$. As describe in Protocol~\ref{protocol:secworst} $S_1$ takes as input $(\pk_\p, E(I), H)$ and $S_2$ takes as input $(\pk_\p, \sk_\p)$.
 When $\SecWorst$ terminates $S_1$ receives the output $\enc(W)$ such that $W$ is the worst score based on the list $H$, and let 
 $\L_{s_1} = (|H|, \EP^d(\ER, q))$, $\L_{s_2} = |\ER|$.
Then $\Pi_{\SecWorst}$ is secure based on the definition~\ref{def:sec-servers}, i.e.,
\begin{align*}
(1). & \Big(\SIM_{s_2}\big(\pk_\p, \L_{s_2}\big), \SecWorst(\pk_\p, \sk_\p, E(I), H) \Big) \approxeq \\ 
  & \ \   \Big(\view^{\SecWorst}_{S_1}(\pk_\p, \sk_\p, E(I), H),  \oput^{\SecWorst}(\pk_\p, \sk_\p ,  E(I), H)\Big)\\
(2). & \Big(\SIM_{s_1}\big(\pk_\p, \sk_\p, \L_{s_1}\big) \approxeq \view_{S_2}^{\SecWorst}(\pk_\p, \sk_\p, E(I), H)\Big)
\end{align*} 

\end{lemma}

\begin{proof}
% During the execution of $\SecWorst$, $S_1$ learns nothing (i.e. $\L_{s_1}(\ER) = \emptyset$), 
% while $S_2$ learns the leakage function $\L_{s_2} = (|L|, \ell_{eq})$,
% where $|L|$ is the total number of the encrypted items, 
% $\ell_{eq}$ is the number of the objects that are the same.
We construct $\SIMtwo$ as follows. $\SIMtwo$ behaves like $S_1$ and interacts with $S_2$.
On the input of the list $H$ and the encrypted item $E(I)$, $\SIMtwo$ 
runs the $\SecWorst$ using the homomorphic properties from $\EHL$ and encryptions and, hence, learns nothing more than what can be already computed from the inputs. 
$\SIMtwo$ simply just follows the $\SecWorst$ protocol. First, $\SIMtwo$ generates the random permutation $\pi$, then sends the encrypted $\enc(b_j)$ to $S_2$ based on the description of the $\SecWorst$ protocol.
When receiving the encrypted bit $\Etwo{t_i})$, $\SIMtwo$ computes the ciphertexts specified in $\SecWorst$. 
$\SIMtwo$ continues by homomorphically computing the $\prod_{i = 1}^{S}\En{x_i'}$.
Finally, based on the protocol $\SecWorst$, $\SIMtwo$ obtains encrypted worst score $\enc(W)$. 
Since all of the messages are encrypted under semantically secure encryption. $\SIMtwo$ learns nothing from the protocol $\SecWorst$.
On the other hand, $\SIMone$, similar as $S_2$, has the access to the keys $\pk_\p$,  $\sk_\p$ and, hence, can decrypt the message received from $S_1$. $\SIMone$ also gets the $\L_{s_1} = (|H|, \EP^d(\ER, q))$ at depth $d$ for some query $q$.
By receiving $\enc(b_i)$ from $S_1$ and gets $\L_{s_1}$, $\SIMone$ can simulates the
views for $S_1$ and behaves exactlly the same as $S_2$. As described in $\SecWorst$, $\SIMone$ sends the $\Etwo{t_i}$ based on the output of $L_{s_1}$. Therefore, $S_1$ cannot distinguish from the transcripts if it is interacting with $S_2$ or $\SIMone$.
For the subroutine $\RecoverEnc$, the privacy for both $S_1$ and $S_2$ is captured similarly by constructing the simulator $\SIMtwo$ and $\SIMone$ for them.
The simulator $\SIMtwo$, as $S_1$, gets the public key $\pk_\p$ and on input of $\Etwo{\enc(c)}$, $\SIMtwo$ pick a random element $r \random \Z_n$, and send $\Etwo{\En{c+r}}$ to $S_2$. Upon receiving $\enc(c')$ from $S_2$, $\SIMtwo$ then computes the $\enc(c')\cdot\enc(-r)$. $S_2$ cannot distinguish if it is interacting with$\SIMtwo$ or $S_1$ since the semantic security of encryption. Similarly, $\SIMone$ who holds the secret key $\sk_\p$, simply just follow $\RecoverEnc$ by decrypting the $\Etwo{\enc(c+r)}$ and sends back $\enc(c+r)$. 
During the execution of $\RecoverEnc$, neither $S_1$ or $S_2$ can distinguish if they interact with the real server or the simulator because of the semantic secure encryption scheme.
\end{proof}

\ignore{
\section{Architecture and Security Model}
\begin{definition}\label{def:secquery}
Let $\Pi_\q$ be an encrypted scheme that can support query type $\q$. 
$\Pi_\q$ consists of an algorithms $\setup$, $\token$, and a protocol $\query$ between the client 
and two non-colluding servers $S_1$ and $S_2$. In particular,
\begin{itemize}
\item $(\ER, K)\larr\setup(\lambda, R)$: takes a relation $R$, the security parameter $\lambda$, and outputs a secret key $K$ along with 
	an encrypted database $\ER$. 
\item $(\result, \bot)\larr \query((K, q), \ER)$: is a protocol between a client $C$ and the servers $S_1$ and $S_2$. The client
    $C$ holds the key $K$ and a query $q$, $S_1$ holds an encrypted databases $\ER$, and $S_2$
    holds the secret key $K$. After the execution of the protocol, the client receives the query
    results $\result$, and both servers receive $\bot$. 
\end{itemize}
For the query type $\q$, let $\result'$ be the query result when querying $q$ on the plaintext database $R$. Then we
say the scheme $\Pi_\q$ is correct if for all $\lambda\in\NN$, for all database $R$, and for all query $q$,
$$\Pr\big[ \result = \result' \big] \ge 1 - \negl$$ 
where the probability is over the randomness in computing 
$(\ER, K)\larr\setup(\lambda, R)$ and $(\result, \bot)\larr \query((K, q), \ER)$, and $\negl$ is a
negligible function.
\end{definition}

\begin{definition}\label{def:secquery}
Let $\SecTopK = (\enc, \Token, \SecQuery)$ be a top-$k$ query processing scheme 
and consider the following probabilistic experiments where $\E$ is an environment, 
$\C$ is a client, $S_1$ and $S_2$ are two non-colluding semi-honest servers, 
$\SIM_1$ and $\SIM_2$ are two simulators, and $\L_\setup$, 
$\L_\query = (\L^1_\query, \L^2_\query)$ are (stateful) leakage functions:
\\
\\
\noindent{\bf $\Ideal(1^\lambda)$:} 
\begin{itemize}
 \item The environment $\E$ outputs a relation $R$ of size $n$ and 
 	sends it to the client $\C$. $\C$ submits the relation $R$ 
    to $\Fideal$, i.e. an \textbf{ideal} top-$k$ functionality.
	$\Fideal$ outputs $\L_\setup(R)$ and $1^\lambda$, and gives 
    $\L_\setup(R)$, $1^\lambda$ to $\SIM_1$.
    Given $\L_\setup(R)$ and $1^\lambda$, $\SIM_1$ generates 
    an encrypted relation database $\ER$. 

 \item $\C$ generates a polynomial number of adaptively chosen queries 
    $(q_1,\ldots,q_m)$. For each query $q_i$, $\C$ submits $q_i$ to $\Fideal$, $\Fideal$
    then sends $\L^1_\query(\ER, q_i)$ to $\SIM_1$ and sends $\L^2_\query(\ER, q_i)$
    to $\SIM_2$.
	After the execution of the protocol, $\C$ outputs $\out_\C'$, 
 	$\SIM_1$ outputs $\out_{\SIM_1}$, and $\SIM_2$ outputs $\out_{\SIM_2}$.
\end{itemize}

\noindent {\bf $\Real_{\A}(1^\lambda)$:}
 \begin{itemize}
    \item The environment $\E$ outputs a relation $R$ of size $n$ and 
 	sends it to the client $\C$. 

    \item $\C$ computes $(\k, \ER) \larr \enc(1^\lambda, R)$
          and sends the encrypted relation $\ER$ to $S_1$.

    \item $\C$ generates a polynomial number of adaptively chosen queries $(q_1,\ldots,q_m)$. 
         For each query $q_i$, $\C$ computes the token $\tk_i\larr\Token(K, q_i)$ and sends $\tk_i$
         to $S_1$. $S_1$ run the protocol $\SecQuery\big(\tk_i, \ER\big)$ with $S_2$. 
         After the execution of the protocol, $S_1$ sends the results to $\C$. 
         $\C$ outputs $\out_\C$, 
 		 $S_1$ outputs $\out_{S_1}$, and $S_2$ outputs $\out_{S_2}$.
  \end{itemize}
We say that $\SecQuery$ is adaptively $(\L_\setup,\L_\query)$-semantically secure if the following 
holds:
  \begin{enumerate}
	\item For all $\E$, for all $S_1$, there exists a ppt simulator $\SIM_1$ 
       such that, for all ppt distinguisher $\Dis$,
       \[ 
       		\big|\Pr\left[\Dis(\angles{\out_{S_1}, \out_\C}) = 1\right] - 
		       \Pr\left[\Dis(\angles{\out_{\SIM_1}, \out_\C'}) = 1 \right]\big| = \negl(\lambda).
		\]
	\item For all $\E$, for all $S_2$, there exists a ppt simulator $\SIM_2$ 
		such that, for all ppt distinguisher $\Dis$,
       \[ 
       		\big|\Pr\left[\Dis(\angles{\out_{S_2}, \out_\C}) = 1\right] - 
		       \Pr\left[\Dis(\angles{\out_{\SIM_2}, \out_\C'}) = 1 \right]\big| = \negl(\lambda).
		\]
   \end{enumerate}
   
\end{definition}
}
\end{appendices}
